# Supplementary material for: SAVME: Efficient Safety Validation for Autonomous Systems Using Meta-Learning
Source: arXiv:2309.12474 source file (2023-09-30)
Supplement: Supplementary file 1 [file appendix.tex]

\section*{\textsc{Appendix}}

IN CASE WE ACTUALLY HAVE ANY APPENDICIES
